# Supplementary material for: Motivic Integration and Logarithmic Geometry
Source: arXiv:1505.05688 source file (2015-05-21)
Supplement: Supplementary file 1 [file myappendix.tex]

\chapter{This is myappendix}\label{ch:myappendix}

\ldots

\instructionsappendices

%%%%%%%%%%%%%%%%%%%%%%%%%%%%%%%%%%%%%%%%%%%%%%%%%%
% Keep the following \cleardoublepage at the end of this file, 
% otherwise \includeonly includes empty pages.
\cleardoublepage

% vim: tw=70 nocindent expandtab foldmethod=marker foldmarker={{{}{,}{}}}
